# Supplementary material for: Quantum Computed Green's Functions using a Cumulant Expansion of the Lanczos Method
Source: arXiv:2309.09685 source file (2024-06-18)
Supplement: Supplementary file 1 [file appendix1.tex]

\section{} \label{sec:appendix}

% % YXXX Ansatz
% \begin{figure}[ht]
% \centering
% \begin{quantikz}
% \lstick{$\ket{0}$} & \gate{X} & \gate{V} & \qw & \qw & \targ{} & \gate{R_z(-\theta)} & \targ{} & \qw & \qw & \gate{V^{\dagger}} & \qw \\
% \lstick{$\ket{0}$} & \gate{H} & \qw & \qw & \targ{} & \ctrl{-1} & \qw & \ctrl{-1} & \targ{} & \qw & \gate{H} & \qw \\
% \lstick{$\ket{0}$} & \gate{X} & \gate{H} & \targ{} & \ctrl{-1} & \qw & \qw & \qw & \ctrl{-1} & \targ{} & \gate{H} & \qw \\
% \lstick{$\ket{0}$} &  \gate{H} & \qw & \ctrl{-1} & \qw & \qw & \qw & \qw & \qw & \ctrl{-1} & \gate{H} & \qw \\
% \end{quantikz} \\
% \caption{The YXXX ansatz applied to the $|1010\rangle$ reference state.}
% \label{fig:yxxx}
% \end{figure}

% YXXX+YX Ansatz
\begin{figure}[ht]
\centering
\begin{quantikz}
\lstick{$\ket{0}$} & \gate{X} & \gate{V} & \qw & \qw & \targ{} & \gate{R_z(-\theta_2)} & \targ{} & \qw & \qw & \gate{V^{\dagger}} & \gate{V} & \targ{} & \gate{R_z(-\theta_1)} & \targ{} & \gate{V^{\dagger}} & \qw \\
\lstick{$\ket{0}$} & \gate{H} & \qw & \qw & \targ{} & \ctrl{-1} & \qw & \ctrl{-1} & \targ{} & \qw & \gate{H} & \qw & \qw & \qw & \qw & \qw & \qw \\
\lstick{$\ket{0}$} & \gate{H} & \qw & \targ{} & \ctrl{-1} & \qw & \qw & \qw & \ctrl{-1} & \targ{} & \gate{H} & \gate{H} & \ctrl{-2} & \qw & \ctrl{-2} & \gate{H} & \qw \\
\lstick{$\ket{0}$} & \gate{X} & \gate{H} & \ctrl{-1} & \qw & \qw & \qw & \qw & \qw & \ctrl{-1} & \gate{H} & \qw & \qw & \qw & \qw & \qw & \qw \\
\end{quantikz} \\
\caption{The YXXX+YX ansatz applied to the $|1001\rangle$ reference state.}
\label{fig:yxxx+yx}
\end{figure}

\newpage
% \begin{landscape}
% YXXX+YX Ansatz SHORTER
\begin{sidewaysfigure}[ht]
\centering
\begin{quantikz}
\lstick{$\ket{0}$} & \gate{X} & \gate{S^{\dagger}} & \gate{V^{\dagger}} & \targ{} & \qw & \gate{R_z(\theta_2)} & \qw & \targ{} & \gate{V} & \gate{S} & \ctrl{3} & \qw & \gate{V} & \qw & \targ{} & \gate{R_z(\theta_1)} & \targ{} & \gate{V^{\dagger}} & \qw & \qw \\
\lstick{$\ket{0}$} & \qw & \qw & \qw & \qw & \qw & \qw & \qw & \qw & \qw & \targ{} & \qw & \qw & \qw & \qw & \qw & \qw & \qw & \qw & \qw & \qw \\
\lstick{$\ket{0}$} & \gate{V} & \qw & \qw & \ctrl{-2} & \gate{H} & \gate{R_z(-\theta_2)} & \gate{H} & \ctrl{-2} & \gate{V^{\dagger}} & \ctrl{-1} & \qw & \qw & \gate{H} & \qw & \ctrl{-2} & \qw & \ctrl{-2} & \gate{H} & \qw & \qw \\
\lstick{$\ket{0}$} & \qw & \qw & \qw & \qw & \qw & \qw & \qw & \qw & \qw & \qw & \targ{} & \qw & \qw & \qw & \qw & \qw & \qw & \qw & \qw & \qw \\
\end{quantikz} \\
\caption{The YXXX+YX ansatz applied to the $|1001\rangle$ reference state.}
\label{fig:yxxx+yx_short}
\end{sidewaysfigure}
% \end{landscape}

% % HEA ansatz circuit
% \begin{figure}[h]
% \centering
% \begin{quantikz}
% \lstick{$\ket{0}$} &  \gate{R_y(\theta_0)} &\ctrl{1} \gategroup[4,steps=4,style={dashed,
% rounded corners,fill=blue!20, inner xsep=3.5pt},
% background,label style={label position=below,anchor=
% north,yshift=-0.2cm}]{{ x d}} & \qw & \qw &\gate{R_y(\theta_4)} &\qw  \\
% \lstick{$\ket{0}$} &  \gate{R_y(\theta_1)}  & \targ{}  & \ctrl{1} &\qw &\gate{R_y(\theta_5)} & \qw \\
% \lstick{$\ket{0}$} &  \gate{R_y(\theta_2)}  & \qw & \targ{} & \ctrl{1}  & \gate{R_y(\theta_6)} & \qw \\
% \lstick{$\ket{0}$} &  \gate{R_y(\theta_3)}  & \qw & \qw & \targ{} & \gate{R_y(\theta_7)} & \qw
% \end{quantikz} \\
% \caption{The hardware efficient RY-ansatz for 4 qubits with d layers.}
% \label{fig:hea}
% \end{figure}
